# Supplementary material for: WASP-4 transit timing variation from a comprehensive set of 129 transits
Source: arXiv:2004.09109 source file (2020-04-20)
Supplement: Supplementary file 1 [file wasp4_suppl.pdf]

MNRAS 000, 1–1 (2020) Preprint 17 April 2020 Compiled using MNRAS LATEX style file v3.0

# WASP-4 transit timing variation from a comprehensive set of 129 transits: online-only supplement

R.V. Baluev et al.

17 April 2020

**ABSTRACT**
This file contains some additional figures.

**Key words:** online supplement

## REFERENCES

Baluev R. V., et al., 2019, MNRAS, 490, 1294
Bouma L. G., Winn J. N., Howard A. W., Howell S. B., Isaacson H., Knutson H., Matson R. A., 2020, ApJ, Lett, arXiv:2004.00637

This paper has been typeset from a TEX/LATEX file prepared by the author.

© 2020 The Authors

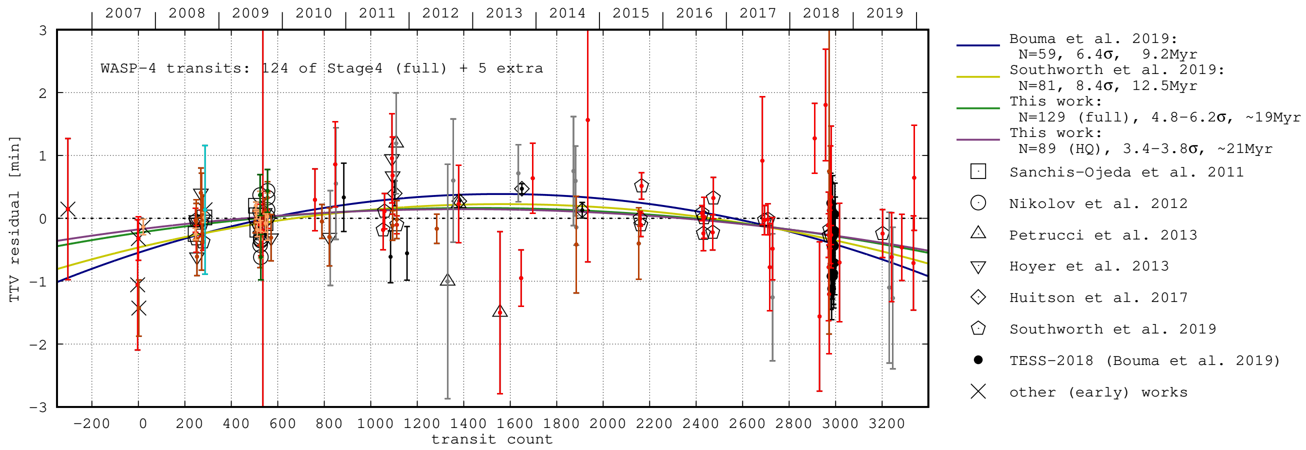


**Figure 1.** Transit times of WASP-4 (full dataset) and several models of the quadratic TTV trend. Point colors correspond to different spectral filters (legend omitted, same as in Baluev et al. 2019). Point shapes refer to different literature sources (given in the legend). Points without a special symbol are amateur observations. The magnitude of the trend, its significance (depending on the noise model), and additional information, are also given at the legend.

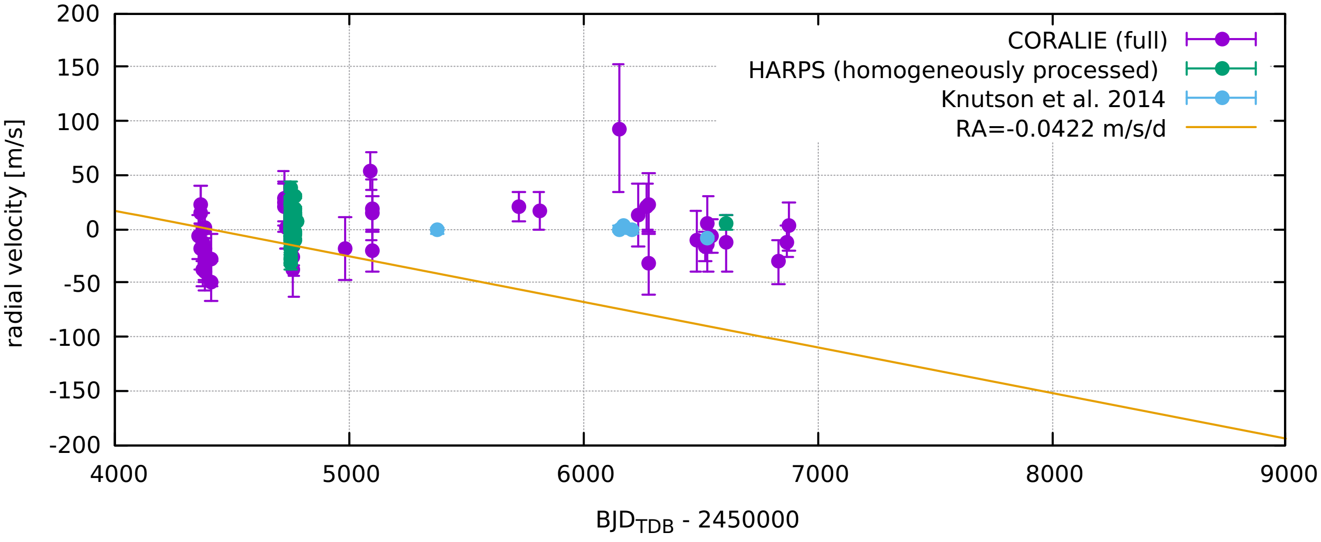


**Figure 2.** Radial velocities of WASP-4 from (Baluev et al. 2019), compared with the radial acceleration of $-0.0422$ m s$^{-1}$d$^{-1}$, or $-15.4$ m s$^{-1}$yr$^{-1}$, from (Bouma et al. 2020). The disagreement of this model with full CORALIE and homogeneously derived HARPS data is obvious (notice a single HARPS point to the right). Bouma et al. (2020) used CORALIE and HARPS data from the left portion of this plot (before JD2455000).
